# Supplementary material for: Spectral analysis of high order continuous FEM for hyperbolic PDEs on triangular meshes: influence of approximation, stabilization, and time-stepping
Source: arXiv:2206.06150 source file (2022-06-13)
Supplement: Supplementary file 1 [file 0_appendix.tex]

\appendix
\section{Appendices}
\textbf{Notation 1:} $\lambda=(\lambda_1,\lambda_2,\lambda_3)$ is the barycentric coordinates relative to the vertices $v_1$, $v_2$ and $v_3$, $\nabla_i = \nabla (\lambda_i), \forall i$, and $\phi_p$ is the basis function which correspond to the degree of freedom $p$. We pose (i,j,k) an arbitrary permutation of $(1,2,3)$. \\
Then, $e_{ij}$ corresponds to a node on the edge $[v_i,v_j]$, which is not a vertex (in green on \ref{fig:mesh_elment2} and \ref{fig:cubature_mesh2}), and finally $G$ corresponds to a node in the triangle (in magenta on \ref{fig:mesh_elment2} and \ref{fig:cubature_mesh2}). \\

\textbf{Notation 2: } $w_v$, $w_\alpha$ and $w_\beta$ are weights of respectively vertices , on edges and for the centroid points. For each basis function $\phi$ relative to a DOF, the corresponding weight represents $\int_K \phi$ with $K$ the triangle of reference. It is as well the weight used in quadradrature formula. 

\subsection{Basic triangular elements, definition of basis functions} \label{appendix_lag_bf}
Below are represented classical/basic finite elements: 
\begin{figure}[H]
    \centering
    \includegraphics[width=12cm]{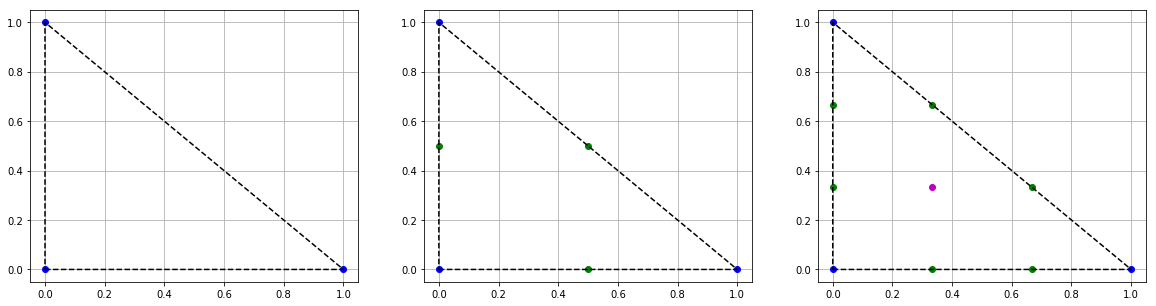}
    \caption{Standar elements $\mathbb{P}_1$ on the left, $\mathbb{P}_2$ on the center and $\mathbb{P}_3$ on the right}
    \label{fig:mesh_elment2}
\end{figure}

\subsubsection*{$\P_1$ element}
The $\mathbb{P}_1$ element contains $3$ degree of freedom: at each vertices $v_1$ , $v_2$ and $v_3$. 
\begin{equation*}
    \quad w_v = \frac{1}{3}
\end{equation*}
with $w_v$ weight of vertices. \\
And then, corresponding basis functions are 
\begin{itemize}
	\item At each vertices $v_1$, $v_2$ and $v_3$. 
	\begin{equation*}
	\hspace*{-1cm}
    \phi_{v_i}(\lambda) = \lambda_i, \qquad \mbox{and} \qquad \nabla \phi_{v_i}(\lambda) = \nabla_i
    \end{equation*}
\end{itemize}

\subsubsection*{$\P_2$ element}
The $\mathbb{P}_2$ element contains $6$ degree of freedom: $3$ at each vertices $v_1$, $v_2$ and $v_3$ and $3$ on edges $(e_{ij},e_{jk},e_{ki})$ (midpoint of edge $[v_i,v_j]$, etc). Respectively, at vertices and midpoints we have those following weights:
\begin{equation*}
    \quad w_v = 0, \quad w_\alpha = \frac{1}{3}
\end{equation*}
And then, corresponding basis functions are 
\begin{itemize}
	\item At vertices of the triangle:
	\begin{equation*}
	\hspace*{-1cm}
    \phi_{v_i}(\lambda) = \lambda_i ( 2\lambda_i-1) , \qquad \mbox{and} \qquad \nabla \phi_{v_i}(\lambda) = \nabla_i (4\lambda_i-1)
    \end{equation*}
	\item On edges:
	\begin{equation*}
	\hspace*{-1cm}
    \phi_{e_{ij}}(\lambda) =  4 \lambda_i \lambda_j , \qquad \mbox{and} \qquad \nabla \phi_{e_{ij}}(\lambda) = 4(\nabla_j \lambda_i + \nabla_i \lambda_j)
    \end{equation*}
\end{itemize}

\subsubsection*{$\P_3$ element} 
The $\mathbb{P}_3$ element contains $10$ degree of freedom : $3$ vertices $v_1$, $v_2$ and $v_3$, $6$ on edges\\ $(e_{ji}(\alpha),e_{ij}(\alpha),e_{kj}(\alpha),e_{jk}(\alpha),e_{ik}(\alpha),e_{ki}(\alpha))$, with $e_{ij}(\alpha)$ such as $\lambda_i = \alpha, \lambda_j = (1-\alpha),\lambda_k = 0$ ($\alpha=\frac{1}{3}$) and a centroid point $G$, such as $\lambda_1 = \lambda_2 = \lambda_3 = \frac{1}{3}$.
\begin{equation*}
    \quad w_v = \frac{1}{30}, \quad w_\alpha = \frac{3}{40}, \quad w_\beta = \frac{9}{20}
\end{equation*}
with $w_v$, $w_\alpha$ and $w_\beta$ weights of respectively vertices, on edges and for the centroid point. \\
And then, corresponding basis functions are 
\begin{itemize}
	\item At vertices of the triangle:
	\begin{equation*}
	\hspace*{-1cm}
    \phi_{v_i}(\lambda) = \frac{1}{2} \lambda_i ( 3 \lambda_i-1)(3\lambda - 2) , \qquad \mbox{and} \qquad \nabla \phi_{v_i}(\lambda) = \frac{1}{2} \nabla_i (9\lambda_i(3\lambda_i-2)+2)
    \end{equation*}
	\item On edges:
	\begin{equation*}
	\hspace*{-1cm}
    \phi_{e_{ij}(\alpha)}(\lambda) =  \frac{9}{2} \lambda_i \lambda_j (3 \lambda_i-1) , \qquad \mbox{and} \qquad \nabla \phi_{e_{ij(\alpha)}}(\lambda) = \frac{9}{2} \left( \nabla_i \lambda_j (6\lambda_i-1)+\nabla_j \lambda_i(3\lambda_i-1) \right)
    \end{equation*}
	\item On the barycentric point:
	\begin{equation*}
   \phi_{G}(\lambda) = 27 \lambda_i \lambda_j \lambda_k, \qquad \mbox{and} \qquad \nabla \phi_{G}(\lambda) = 27 ( \nabla_i \lambda_j \lambda_k + \lambda_i \nabla_j \lambda_k +\lambda_i \lambda_j \nabla_k)
    \end{equation*}
\end{itemize}

\subsection{Cubature elements, definition of basis functions} \label{appendix_cohen_bf}
Below are represented cubature finite elements: 
\begin{figure}[H]
    \centering
    \hspace*{-1cm}
    \includegraphics[width=12cm]{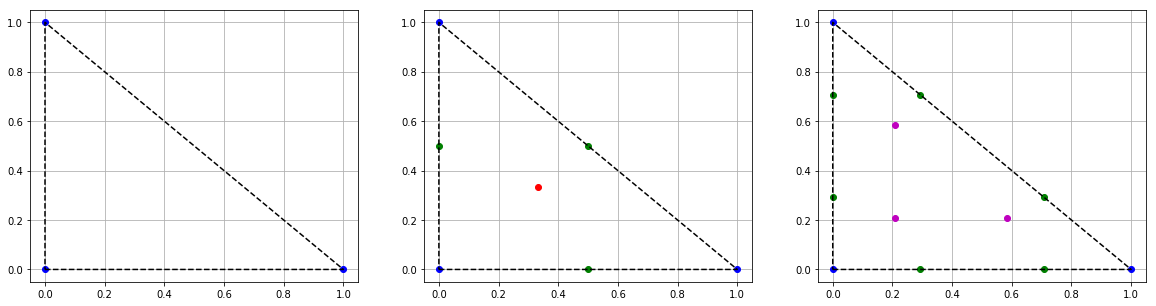}
    \caption{Cohen elements $\Tilde{\mathbb{P}}_1$, $\Tilde{\mathbb{P}}_2$ and $\Tilde{\mathbb{P}}_3$}
    \label{fig:cubature_mesh2}
\end{figure}

\subsubsection*{$\Tilde{\P}_1$ element} 
The $\Tilde{\mathbb{P}}_1$ element contains $3$ degree of freedom: at each vertices $v_1$ , $v_2$ and $v_3$. 
\begin{itemize}
	\item At vertices of the triangle:
	\begin{equation*}
	\hspace*{-1cm}
    \phi_{v_i}(\lambda) = \frac{1}{2} \lambda_i ( 3 \lambda_i-1)(3\lambda - 2) , \qquad \mbox{and} \qquad \nabla \phi_{v_i}(\lambda) = \frac{1}{2} \nabla_i (9\lambda_i(3\lambda_i-2)+2)
    \end{equation*}
\end{itemize}
Corresponding weights are $w_{v_i} = \frac{1}{3}$. And we write $w_v$ the weight for vertices in the triangle. 

\subsubsection*{$\Tilde{\P}_2$ element} 
The $\Tilde{\mathbb{P}}_2$ element contains $7$ degree of freedom: $3$ at each vertices $v_1$, $v_2$ and $v_3$ and $3$ on edges $(e_{ij},e_{jk},e_{ki})$ (midpoint of edge $[v_i,v_j]$, etc) and 1 centroid point $G_\beta$. Respectively, we have those following basis functions and weights:
%\begin{figure}[H]
%    \centering
%    \includegraphics[width=14cm,height=6.5cm]{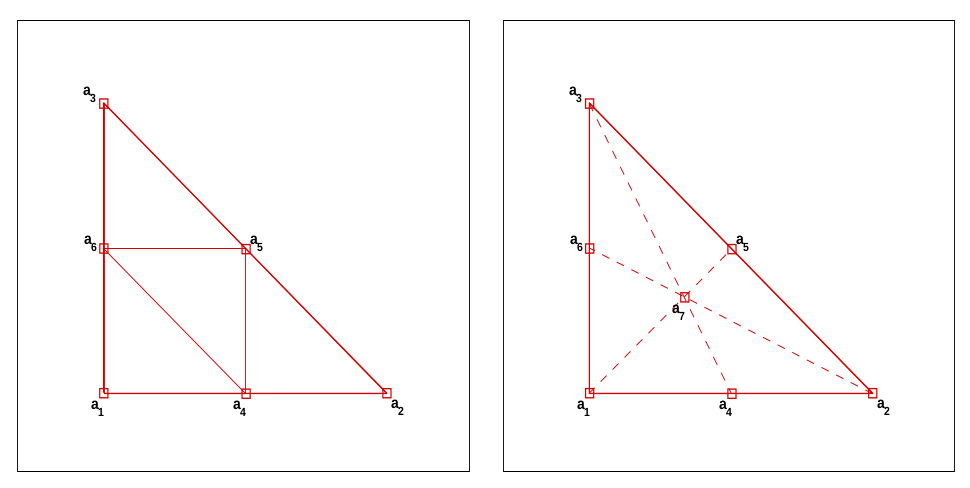}
%    \caption{Santard $\mathbb{P}_2$ at left and cubature $\Tilde{\mathbb{P}}_2$ at right}
%    \label{fig:bas_vs_cond_P2}
%\end{figure}
\begin{itemize}
	\item At vertices of the triangle:
	\begin{equation*}
    \phi_{v_i}(\lambda) = \lambda_i(2\lambda_i-1)+3\lambda_i \lambda_j \lambda_k
    \end{equation*}%, \quad \phi_j(\lambda) = \lambda_j(2\lambda_j-1)+3\lambda_i \lambda_j \lambda_k, \quad \phi_k(\lambda) = \lambda_k(2\lambda_k-1)+3\lambda_i \lambda_j \lambda_k
    \begin{equation*}
        \mbox{and} \quad \nabla \phi_{v_i} = \nabla_i (4\lambda_i-1) + 3( \nabla_i \lambda_j \lambda_k + \lambda_i \nabla_j \lambda_k +\lambda_i \lambda_j \nabla_k)
    \end{equation*}
	\item On edges: 
	\begin{equation*}
    \phi_{e_{ij}}(\lambda) = 4 \lambda_i \lambda_j (1-3 \lambda_k), \quad \phi_{e_{jk}}(\lambda) = 4 \lambda_j \lambda_k (1-3 \lambda_i) , \quad \phi_{e_{ki}}(\lambda) = 4 \lambda_k \lambda_i (1-3 \lambda_j)
    \end{equation*}
    \begin{equation*}
        \mbox{and} \quad \nabla \phi_{e_{ij}} = 4((\nabla_i \lambda_j + \lambda_j \nabla_j)(1-3\lambda_k)-3\nabla_k \lambda_i \lambda_j)
    \end{equation*}    
	\item On the centroid point:
	\begin{equation*}
    \phi_{G_\beta}(\lambda) = 27 \lambda_i \lambda_j \lambda_k, \mbox{and} \qquad \nabla \phi_{G_\beta}(\lambda) = 27 ( \nabla_i \lambda_j \lambda_k + \lambda_i \nabla_j \lambda_k +\lambda_i \lambda_j \nabla_k)
    \end{equation*}
\end{itemize}
with $e_{ij}$ define such as $\lambda_i = \frac{1}{2}$, $\lambda_j = \frac{1}{2}$ and $\lambda_k =0$, the midpoint between vertices $v_i$ and $v_j$, and $G_\beta = (\frac{1}{3} ,\frac{1}{3} ,\frac{1}{3} )$, the barycentre of the triangle. \\
We define $w_v$ the weight at vertices of the triangle, $w_\alpha$ the weight on edges, and $w_\beta $ the weight for barycentric point. \\
Corresponding weights are $w_v = \frac{1}{20}$, $w_\alpha = \frac{2}{15}$ and $w_\beta = \frac{9}{20}$ 

\subsubsection*{$\Tilde{\P}_3$ element}
The $\mathbb{P}_3$ element contains $12$ degree of freedom : $3$ vertices $v_1$, $v_2$ and $v_3$, $6$ on edges\\ $(e_{ji}(\alpha),e_{ij}(\alpha),e_{kj}(\alpha),e_{jk}(\alpha),e_{ik}(\alpha),e_{ki}(\alpha))$, with $e_{ij}(\alpha)$ such as $\lambda_i = \alpha, \lambda_j = (1-\alpha),\lambda_k = 0$ ($\alpha = \frac{-15\sqrt{7}-21+\sqrt{168+174\sqrt{7}}}{2(-15\sqrt{7}-21)}$) and three centroid points $(G_i(\beta),G_j(\beta),G_k(\beta))$, with $G_i(\beta)$ such as $\lambda_i = \beta , \lambda_j = \frac{1-\beta}{2} , \lambda_k = \frac{1-\beta}{2} $, $\beta=\frac{1}{3}+\frac{2\sqrt{7}}{21}$. \\
Respectively, we have those following basis functions and weights:
%\begin{figure}[H]
%    \centering
%    \includegraphics[width=14cm,height=6.5cm]{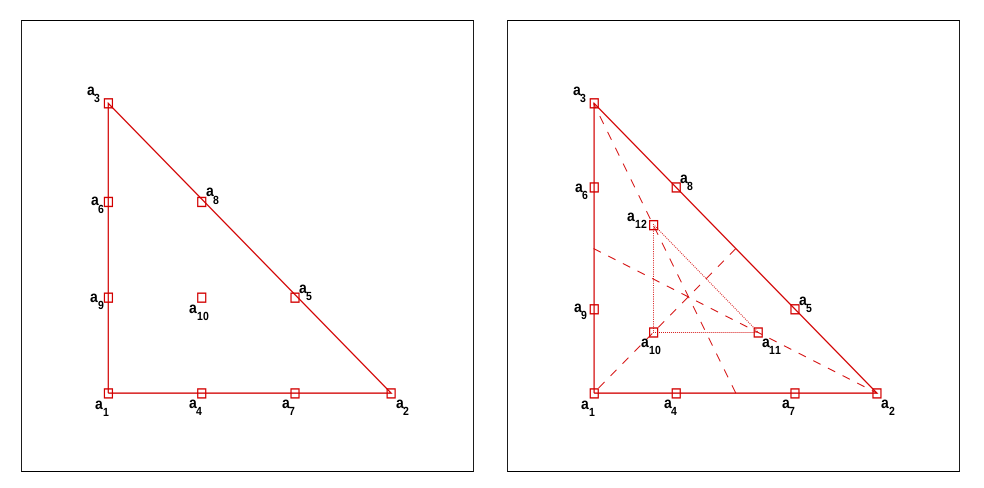}
%    \caption{Santard $\mathbb{P}_3$ at left and cubature $\Tilde{\mathbb{P}}_3$ at right}
%    \label{fig:bas_vs_conv_P3}
%\end{figure}
\begin{itemize}
	\item At vertices of the triangle:
	\begin{align*}
    \phi_{v_i}(\lambda) = & \underbrace{ \lambda_i \left( \sum_l \lambda_l^2 - \frac{1-2\alpha + \alpha^2}{\alpha(1-\alpha)}\lambda_i(\lambda_j+\lambda_k)+ A_{02} \lambda_j \lambda_k \right) }_{p_{i}(\lambda)} \\
    & - \frac{8}{\beta (1-\beta)^2 (3\beta-1)} \lambda_i \lambda_j \lambda_k \left( \sum_{j} b_l (\lambda_l - \frac{1-\beta  }{2}) \right) 
    \end{align*}
    with $b_l = p_{i}(G_l)$. \\
    As $w_i = \frac{1}{|K|}\int_K  \phi_i(\lambda) ds  $, we obtain
    \begin{equation*}
    \hspace*{-1cm}
    A_{02} = \left( w_s -\frac{1}{10}-\frac{1}{15} \left(1- \frac{1-2\alpha + \alpha^2}{\alpha(1-\alpha)} \right) - \frac{1}{90}\frac{8}{\beta (1-\beta)^2 (3\beta-1)}( p_{i}(G_i) +  p_{i}(G_j) +  p_{i}(G_k))      \right) \times \left( \frac{360}{6+\frac{8(1-\beta^2)  }{\beta (1-\beta)^2 (3\beta-1)}} \right)
    \end{equation*}
    And
    \begin{align*}
	\hspace*{-1cm}
         \nabla \phi_{v_i}(\lambda)  =  &\nabla_i \left(\sum_l \lambda_l^2 - \frac{1-2\alpha + \alpha^2}{\alpha(1-\alpha)}\lambda_i(\lambda_j+\lambda_k)+ A_{02} \lambda_j \lambda_k \right) \\
         &  + \lambda_i \left( \sum_l 2\lambda_l \nabla_l - \frac{1-2\alpha + \alpha^2}{\alpha(1-\alpha)} \nabla_i(1-2 \lambda_i) + A_{02} (\nabla_j \lambda_k + \lambda_j \nabla_k)  \right) \\
         \hspace*{-2.5cm}
         & - \frac{8}{\beta (1-\beta)^2 (3\beta-1)} \left[ (\nabla_i \lambda_j \lambda_k + \lambda_i \nabla_j \lambda_k +\lambda_i \lambda_j \nabla_k) \left( \sum_{1\leq l \leq 3} b_l \left( \lambda_l -\frac{1-\beta}{2} \right) \right)+\lambda_i \lambda_j \lambda_k \nabla_i \left( \sum_{1\leq l \leq 3} b_l \nabla_l \right) \right] 
    \end{align*}
	\item On edges: $(e_{ji}(\alpha),e_{ij}(\alpha),e_{kj}(\alpha),e_{jk}(\alpha),e_{ik}(\alpha),e_{ki}(\alpha))$, \\
	with $e_{ij}(\alpha)$ such as $\lambda_i = \alpha, \lambda_j = (1-\alpha),\lambda_k = 0$, and $\alpha = \frac{-15\sqrt{7}-21+\sqrt{168+174\sqrt{7}}}{2(-15\sqrt{7}-21)}$
	\begin{align*}
    \phi_{e_{ij}(\alpha)}(\lambda) = & \underbrace{ \frac{1}{\alpha(1-\alpha)(2\alpha-1)} \lambda_i \lambda_j (\alpha \lambda_i  - (1-\alpha)\lambda_j + (1-2\alpha) \lambda_k)}_{p_{ij}(\lambda)} \\
    &- \frac{8}{\beta (1-\beta)^2 (3\beta-1)} \lambda_i \lambda_j \lambda_k \left( \sum_{j} b_l (\lambda_l - \frac{1-\beta  }{2}) \right) 
    \end{align*}
    with $b_l = p_{ij}(G_l)$, and
    \begin{align*}
         \hspace*{-2cm}
         \nabla \phi_{e_{ij}(\alpha)}(\lambda) =  \frac{1}{\alpha(1-\alpha)(2\alpha-1)} & \left[ (\nabla_i \lambda_j+\lambda_i \nabla_j)(\alpha \lambda_i-(1-\alpha)\lambda_j+(1-2\alpha)\lambda_k) + \lambda_i \lambda_j (\alpha \nabla_i - (1-\alpha) \nabla_j + (1-2\alpha) \nabla_k \right] \\
         - \frac{8}{\beta (1-\beta)^2 (3\beta-1)} & \left[ (\nabla_i \lambda_j \lambda_k + \lambda_i \nabla_j \lambda_k +\lambda_i \lambda_j \nabla_k) \left( \sum_{1\leq l \leq 3} b_l \left( \lambda_l -\frac{1-\beta}{2} \right) \right)+\lambda_i \lambda_j \lambda_k \nabla_i \left( \sum_{1\leq l \leq 3} b_l \nabla_l \right) \right] 
    \end{align*}
	\item On the barycentric points :  $(G_i(\beta),G_j(\beta),G_k(\beta))=(a_{10},a_{11},a_{12})$, \\
	with $G_i(\beta)$ such as $\lambda_i = \beta , \lambda_j = \frac{1-\beta}{2} , \lambda_k = \frac{1-\beta}{2} $, $\beta=\frac{1}{3}+\frac{2\sqrt{7}}{21}$.
	\begin{equation*}
    \phi_{G_i(\beta)}(\lambda) = \frac{8}{\beta(1-\beta)^2(3\beta-1)} \lambda_i \lambda_j \lambda_k (\lambda_i-\frac{1-\beta}{2})
    \end{equation*}
    \begin{equation*}
        \mbox{and} \quad \nabla \phi_{G_\beta}(\lambda) =  \frac{8}{\beta(1-\beta)^2(3\beta-1)} \left( (\nabla_i \lambda_j \lambda_k + \lambda_i \nabla_j \lambda_k +\lambda_i \lambda_j \nabla_k) \left(\lambda_i-\frac{1-\beta}{2}\right)+\lambda_i \lambda_j \lambda_k \nabla_i \right)
    \end{equation*}
\end{itemize}

We define $w_v$ the weight at vertices of the triangle, $w_\alpha$ the weight on edges, and $w_\beta $ the weight for barycentric points. \\
Corresponding weight is $w_v = \frac{1369+767\sqrt{7}}{120(859+395\sqrt{7})}$, $w_\alpha = \frac{287+115\sqrt{7}}{40(173+49\sqrt{7})}$ and $w_\beta = \frac{21\sqrt{7}}{40(2\sqrt{7}+1)}$. \\

%\subsection{Non linear Shallow water - conservative form} \label{NLSW_cons_form}
%Considering the system \refp{eq_sv_1}:
%\begin{equation}
%    \left  \{
%    \begin{array}{ll}
%    	\partial_t h + \partial_x (hu) &= 0 \\
%    	\partial_t (hu) + \partial_x (hu^2 +g\frac{h^2}{2} )& = -gh(S_{ox} + S_{fx})
%	\end{array}
%    \right .
%\end{equation}
%We can write the system in a matricial form:
%\begin{equation*}
%	\partial_t U + \partial_x F(U) = S(U) \quad \Leftrightarrow \quad \partial_t U + A \partial_x U = S(U)
%\end{equation*}
%with $
%	A=\begin{pmatrix}
%	0 & 1 \\
%	gh-u^2 & 2u
%	\end{pmatrix}
%	$. \\
%We now compute eigenvalues of $A$:
%\begin{align*}
%|A-XI|&=det \left( \begin{pmatrix}
%a-X & b \\
%c & d-X
%\end{pmatrix} \right) = (a-X)(d-X)-cb \\
%&= X^2 - X(a+d) + (ad-cb) \\
%\Delta &= (a+d)^2-4(ad-cb) = (a-d)^2 + 4cb \\
%\lambda_{\pm} &= \frac{(a+d) \pm \sqrt{\Delta}}{2}
%\end{align*}
%The spectrum of $A$ is $Sp(A)=\{ u + \sqrt{gh}, u - \sqrt{gh} \} $.
